# Supplementary material for: Geometrically-protected reversibility in hydrodynamic Loschmidt-echo experiments
Source: arXiv:1407.1696 source file (2014-07-07)
Supplement: Supplementary file 1 [file supp.pdf]

# Supplementary Information

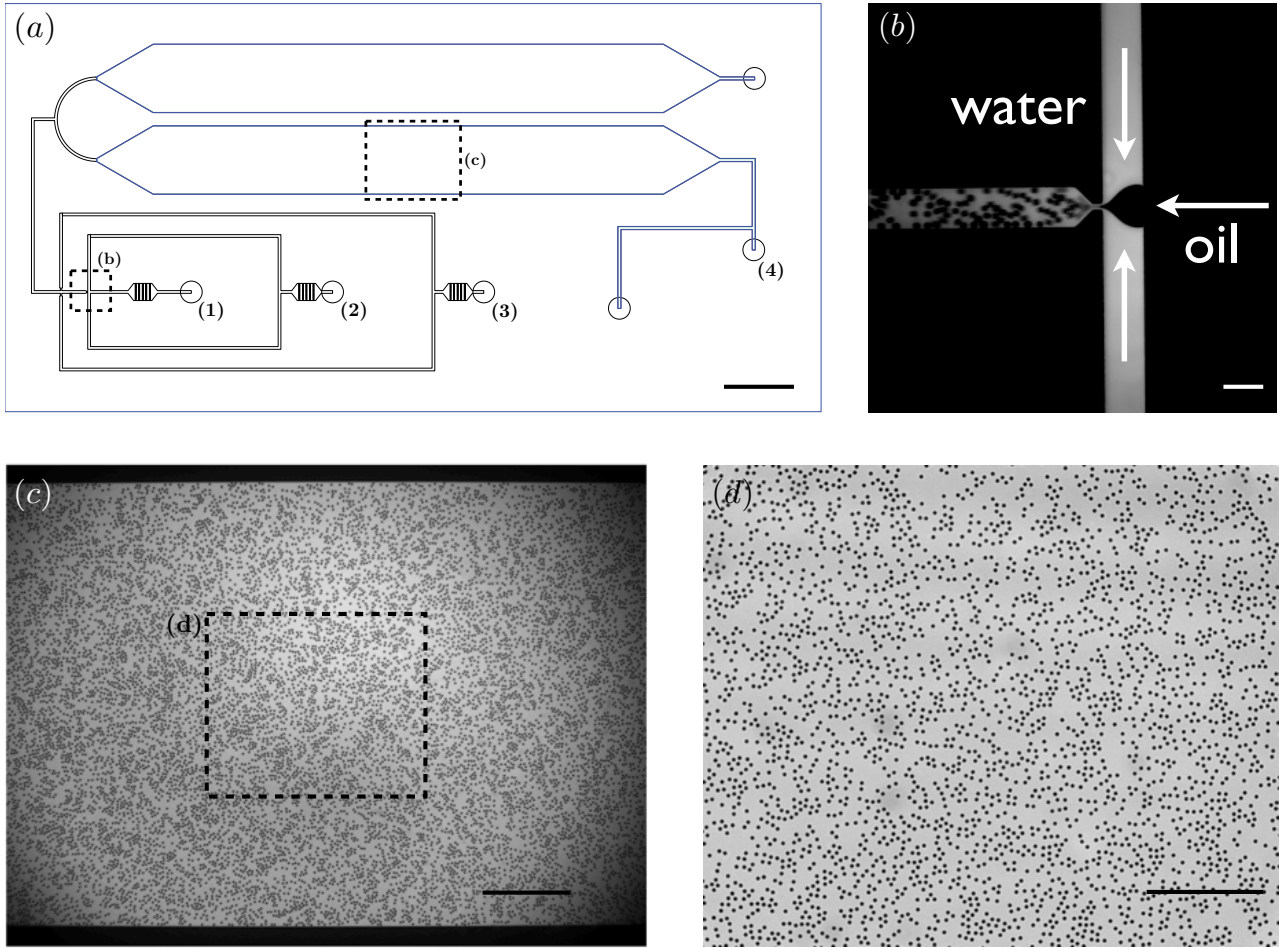

Figure S1:

(a) Schematics of the microfluidic setup. Scale bar: 500  $\mu\text{m}$ . (b) Enlargement on the flow-focusing emitter. Fluorescence imaging picture. Scale bar: 200  $\mu\text{m}$ . (c) Snapshot of the main channel containing the oil-in-water emulsion. Scale bar: 1 mm. (d) Picture of the  $2.70 \times 2.03$  mm observation region where we track the droplets position in time. Scale bar: 500  $\mu\text{m}$ .

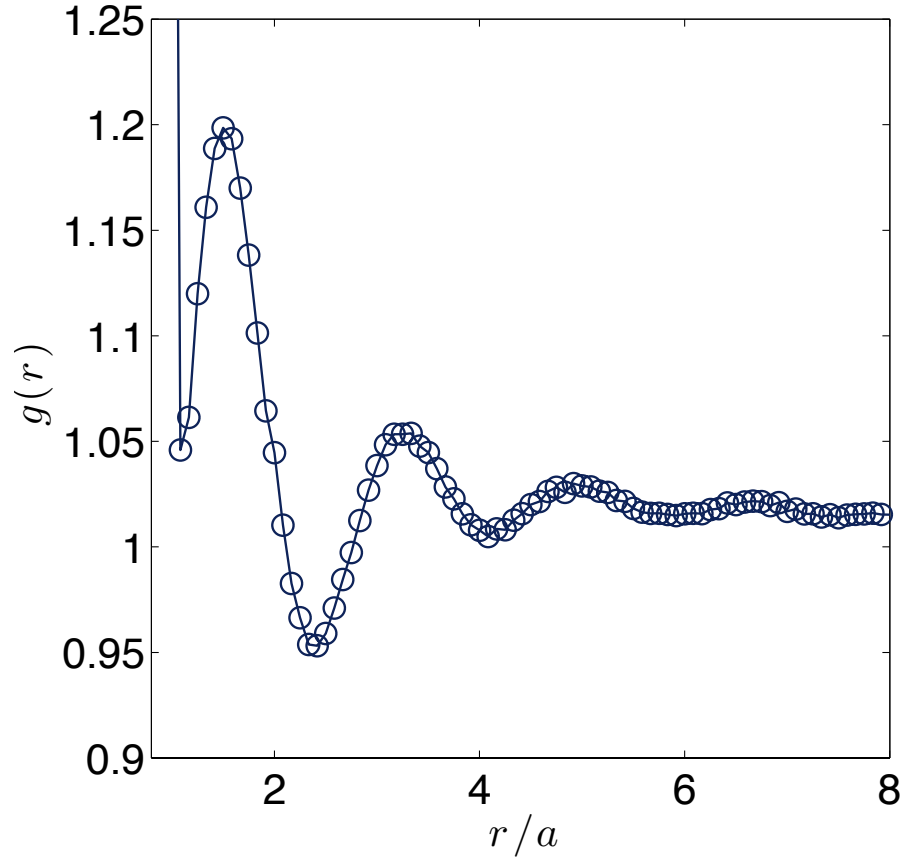

Figure S2:

Close-up on the radial distribution function for  $\Delta=27.9$  a ( $0.99 \Delta^*$ ) to show that the correlation increases up to 7 droplets diameters close to the transition.
